# Supplementary material for: Neural Compression-Based Feature Learning for Video Restoration
Source: arXiv:2203.09208 source file (2022-03-18)
Supplement: Supplementary file 1 [file dehaze_supp.pdf]

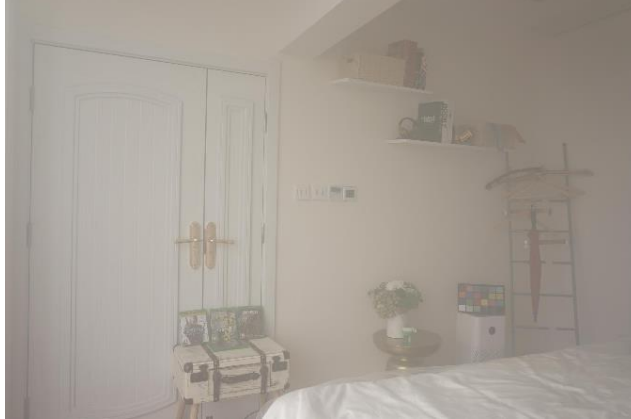

Input

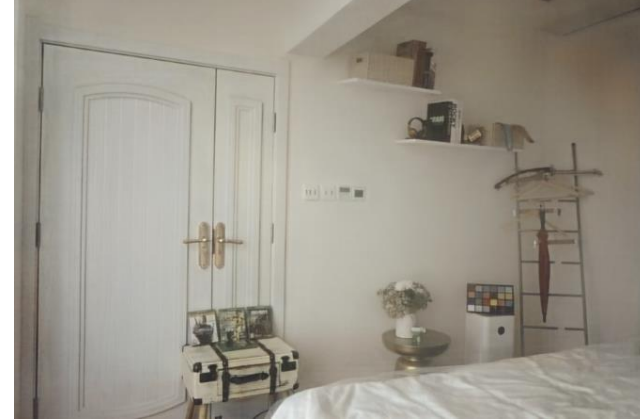

MBSDN

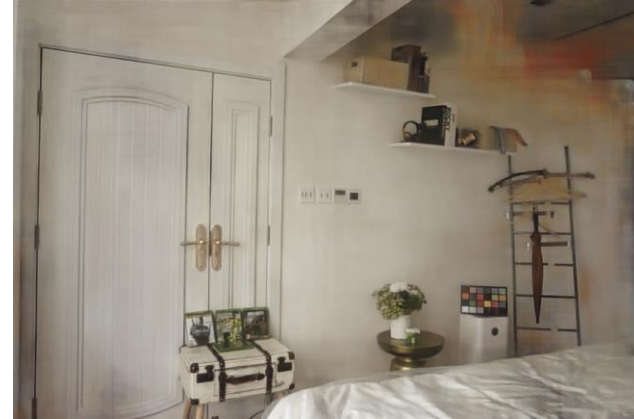

BasicVSR++

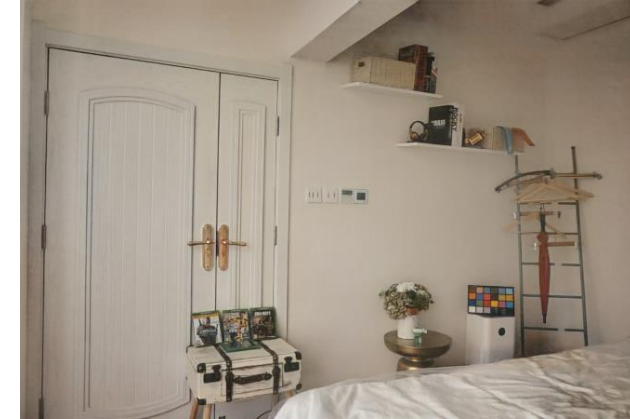

Ours

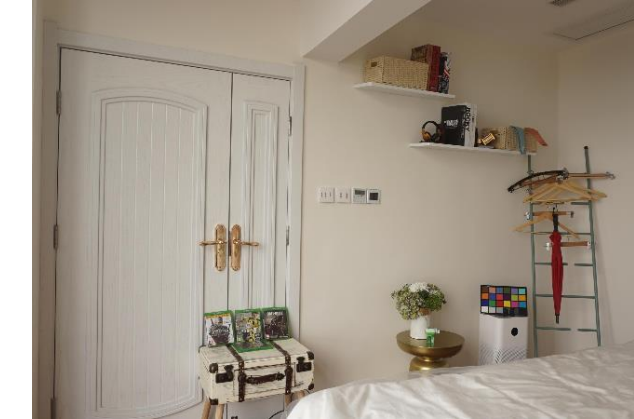

Target

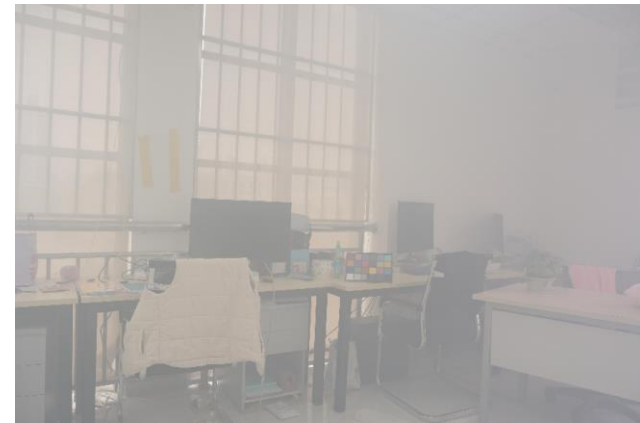

Input

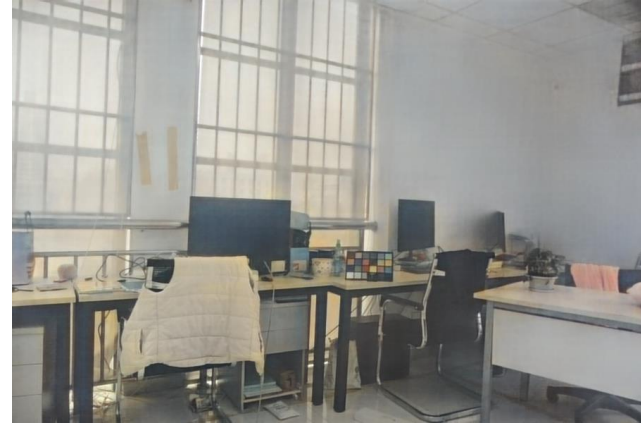

MBSDN

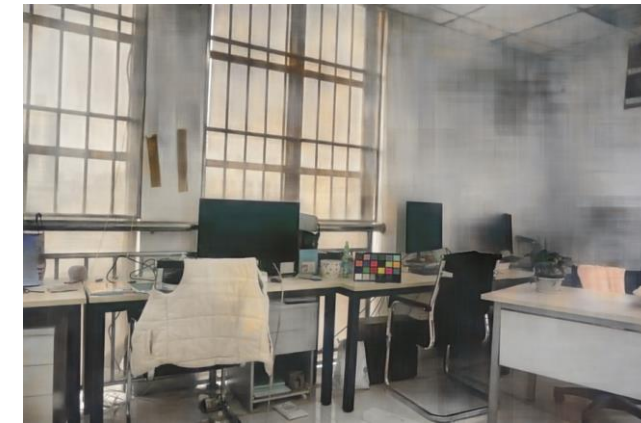

BasicVSR++

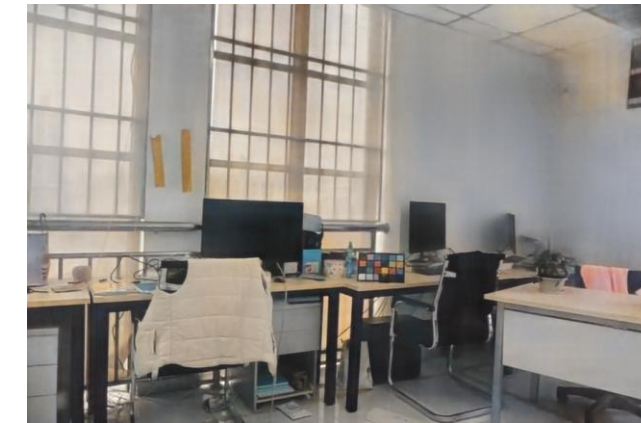

Ours

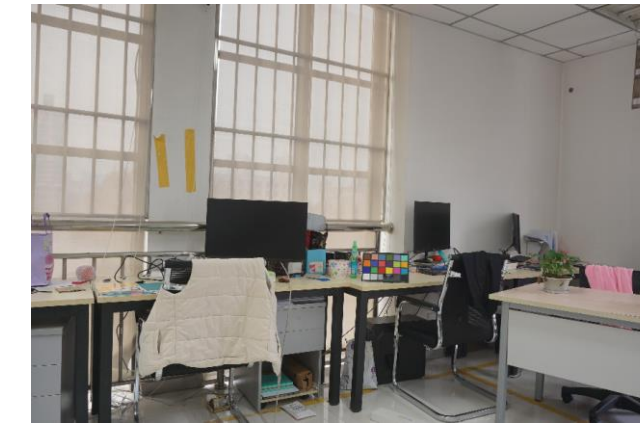

Target
