# Supplementary material for: Neural Compression-Based Feature Learning for Video Restoration
Source: arXiv:2203.09208 source file (2022-03-18)

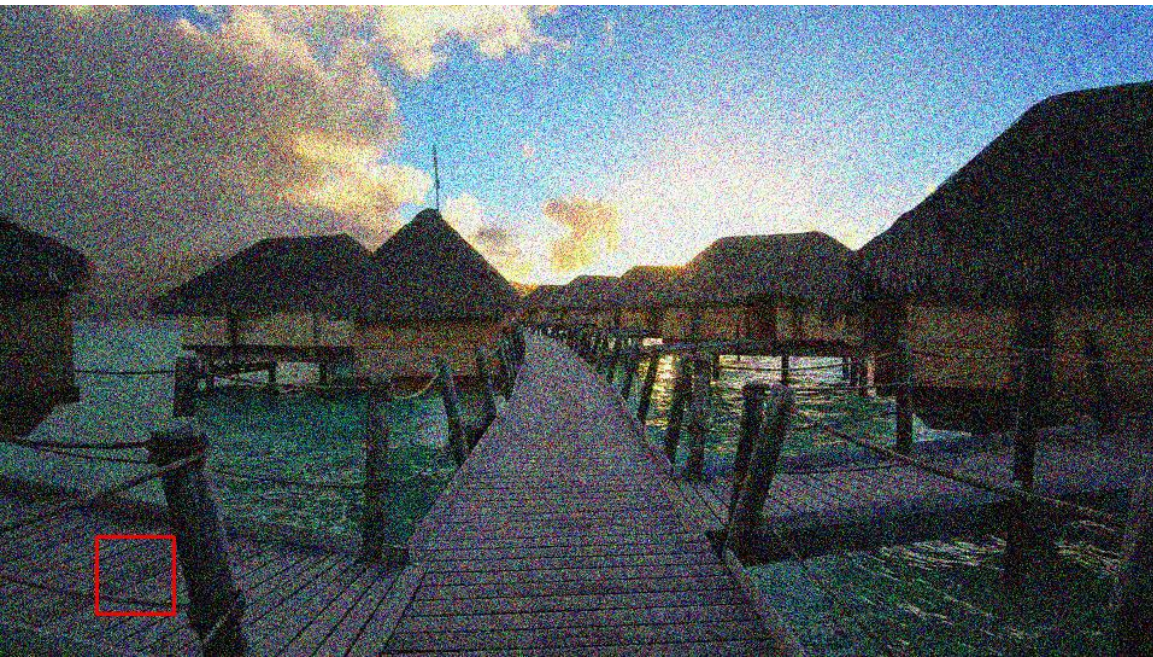

Noisy

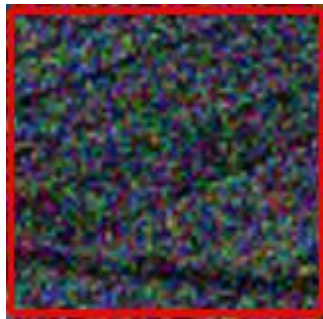

FastDVDNet

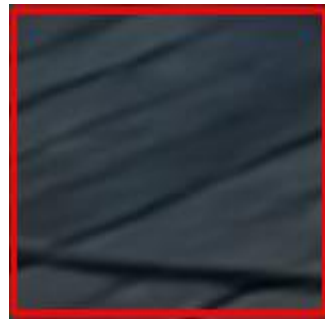

EMVD-L

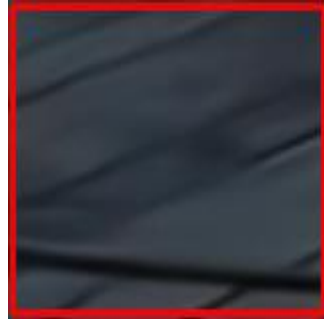

EDVR

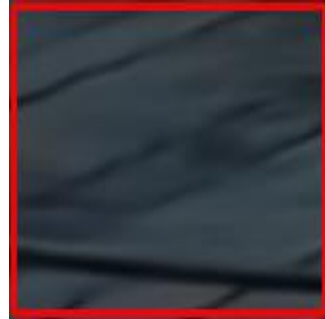

BasicVSR

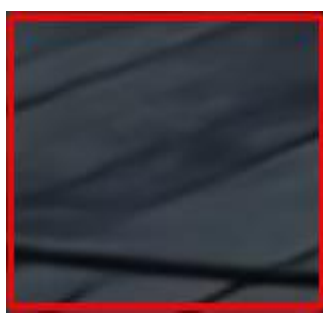

BasicVSR++

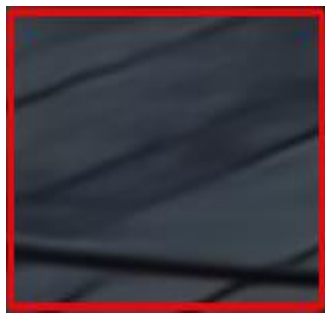

**Ours**

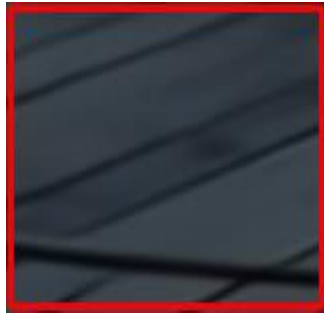

Target

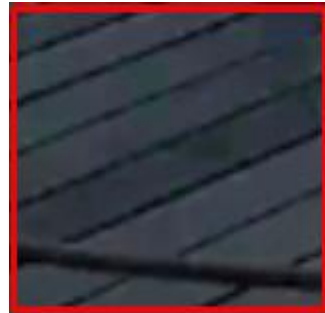

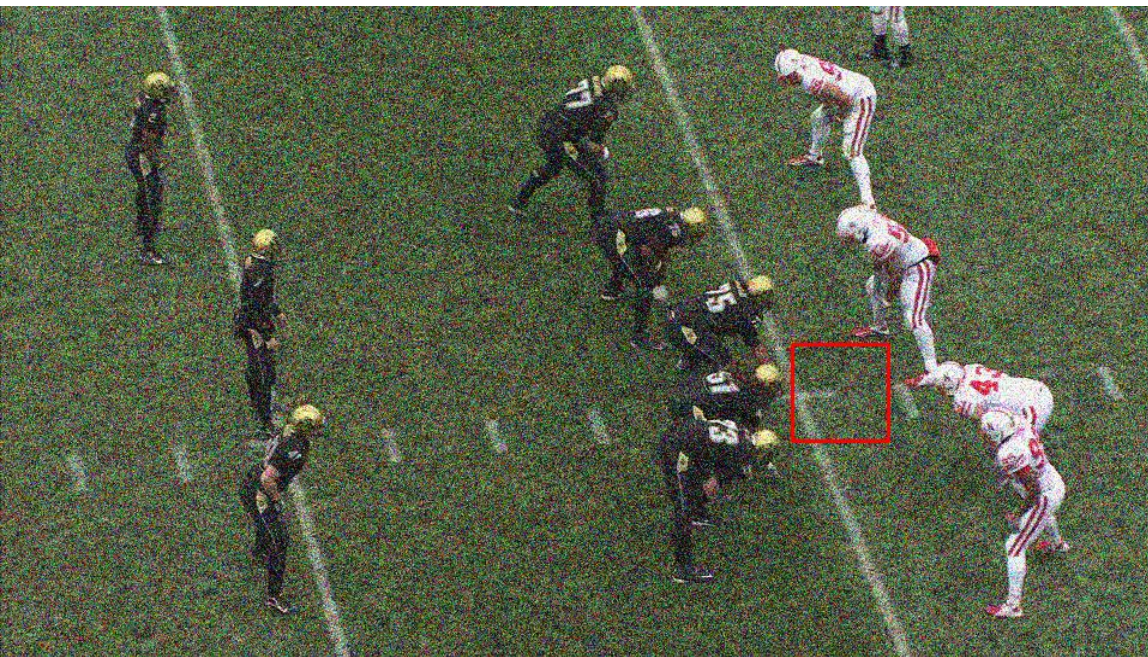

Noisy

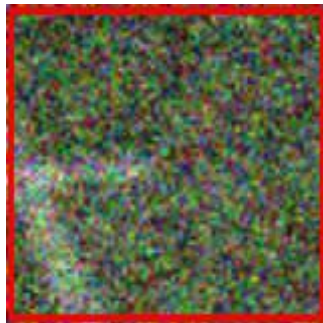

FastDVDNet

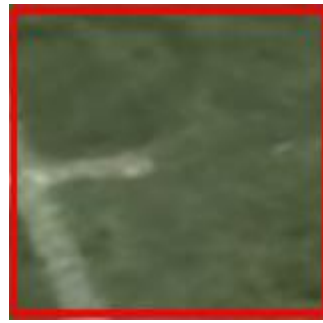

EMVD-L

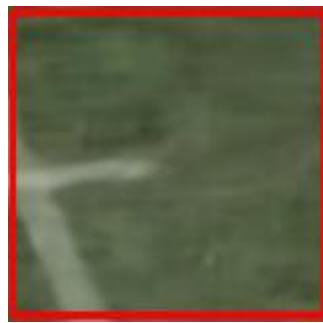

EDVR

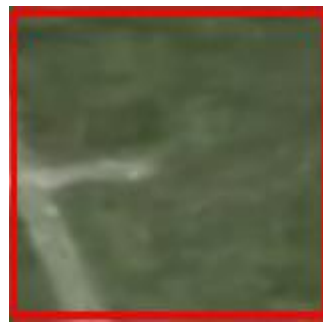

BasicVSR

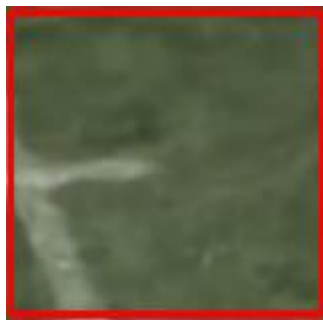

BasicVSR++

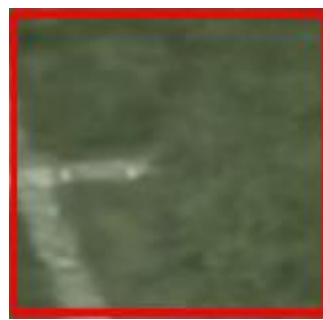

Ours

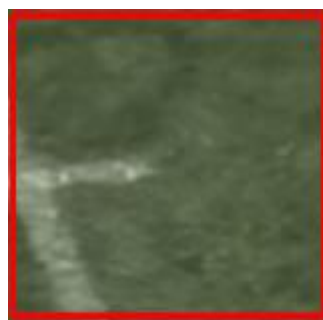

Target

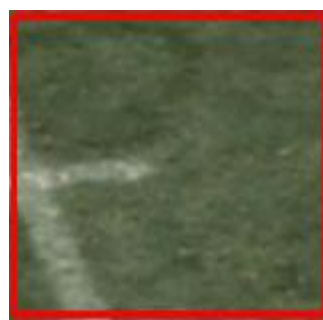

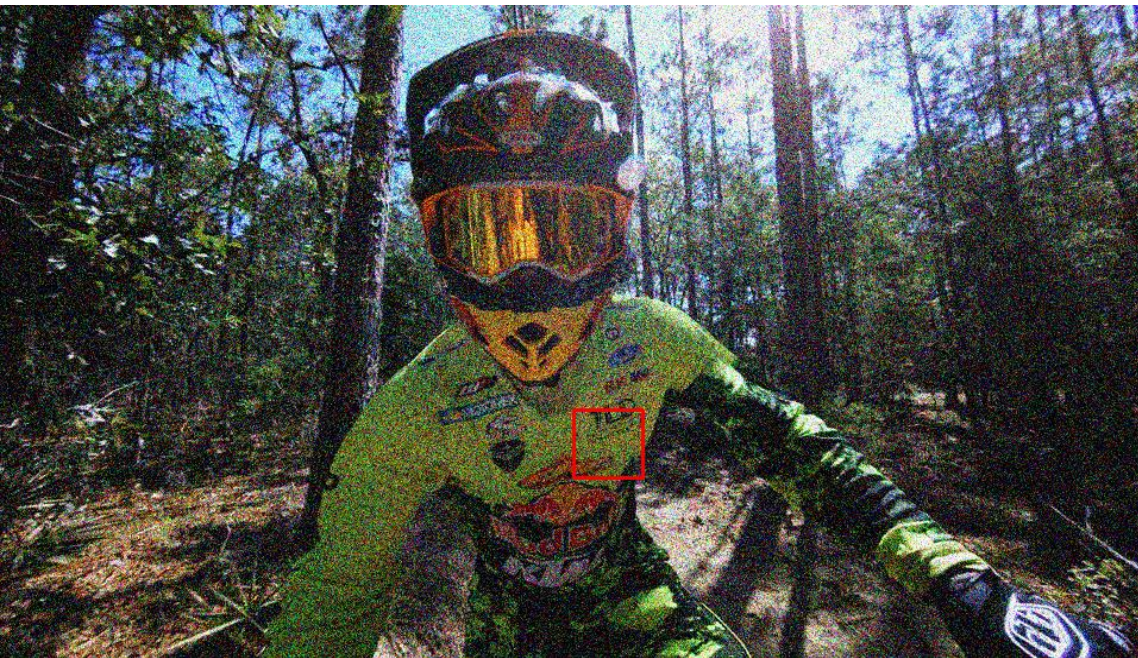

Noisy, 18.8dB

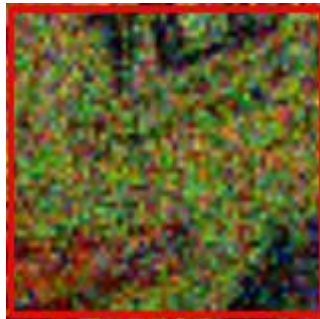

FastDVDNet, 29.7dB

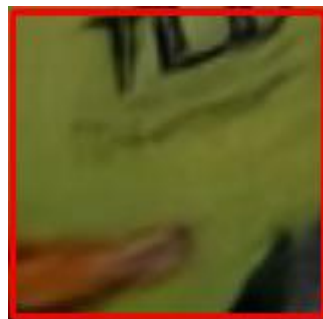

EMVD-L, 29.9dB

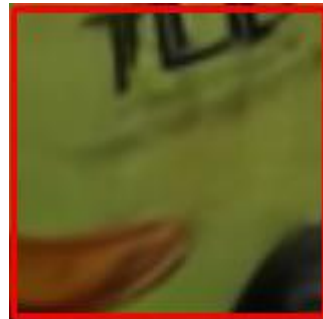

EDVR, 30.5dB

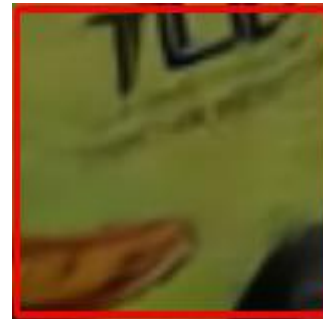

BasicVSR, 30.8dB

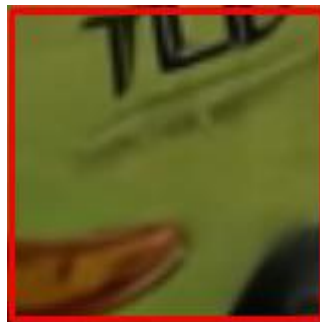

BasicVSR++, 31.4dB

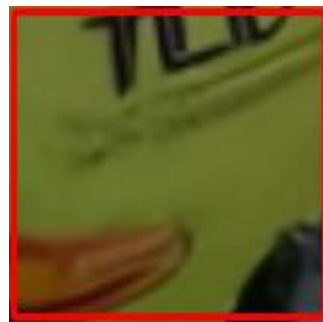

**Ours, 33.4dB**

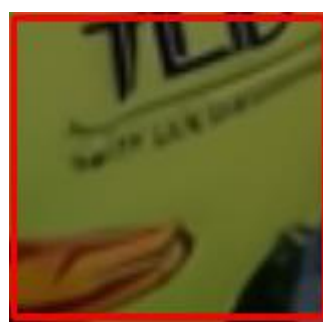

Target

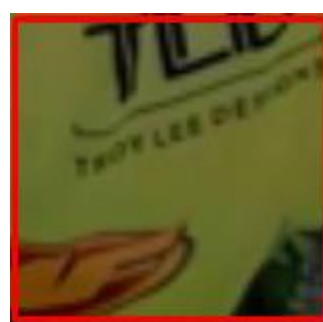

Supplement: Supplementary file 2 [file supp_fig0.pdf]
